# Supplementary material for: Flow-Arrest Transitions in Frictional Granular Matter
Source: arXiv:1810.00043 source file (2019-01-30)
Supplement: Supplementary file 1 [file Suppl.pdf]

# Supplementary Material – Flow-Arrest Transitions in Frictional Granular Matter

Ishan Srivastava,<sup>1</sup> Leonardo E. Silbert,<sup>2</sup> Gary S. Grest,<sup>1</sup> and Jeremy B. Lechman<sup>1</sup>

<sup>1</sup>*Sandia National Laboratories, Albuquerque, New Mexico 87185, USA*

<sup>2</sup>*School of Math, Science, and Engineering,  
Central New Mexico Community College,  
Albuquerque, New Mexico 87106, USA*

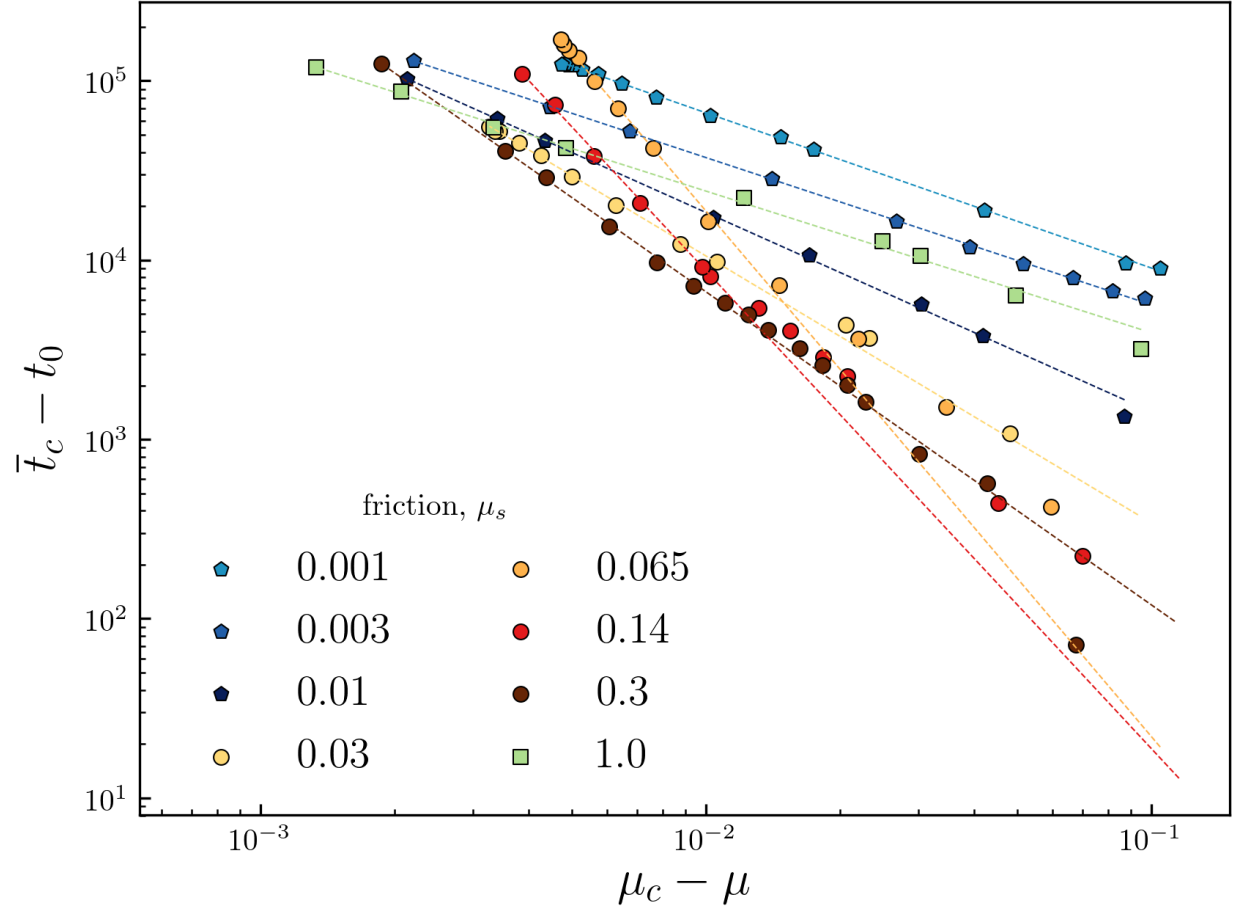

FIG. S1. Log-log plot of  $\bar{t}_c - t_0$  vs.  $\mu_c - \mu$  for eight values of  $\mu_s$  listed in the legend. The dashed lines represent fits to Eq. 1 in the main text.
